# Supplementary material for: Anomalous suppression of large-scale density fluctuations in classical and quantum spin liquids
Source: arXiv:2502.05313 source file (2025-02-07)
Supplement: Supplementary file 1 [file SI.pdf]

# Supplementary Information: Anomalous suppression of large-scale density fluctuations in classical and quantum spin liquids

Duyu Chen,<sup>1,\*</sup> Rhine Samajdar,<sup>2,3,\*</sup> Yang Jiao,<sup>4,5</sup> and Salvatore Torquato<sup>†2,6,7,8</sup>

<sup>1</sup>*Materials Research Laboratory, University of California, Santa Barbara, CA 93106*

<sup>2</sup>*Department of Physics, Princeton University, Princeton, NJ 08544*

<sup>3</sup>*Princeton Center for Theoretical Science, Princeton University, Princeton, NJ 08544*

<sup>4</sup>*Materials Science and Engineering, Arizona State University, Tempe, AZ 85287*

<sup>5</sup>*Department of Physics, Arizona State University, Tempe, AZ 85287*

<sup>6</sup>*Department of Chemistry, Princeton University, Princeton, NJ 08544*

<sup>7</sup>*Princeton Materials Institute, Princeton University, Princeton, NJ 08540*

<sup>8</sup>*Program in Applied and Computational Mathematics, Princeton, NJ 08544*

## CLASSICAL MONOMER-DIMER COVERINGS BELOW MAXIMUM FILLING FRACTION

In this section, we consider classical monomer-dimer coverings on the kagome lattice at filling fractions  $f < 1/4$  (i.e., not all kagome vertices are touched by one dimer), and investigate how the hyperuniformity of the dimer coverings is affected when  $f$  moves away from the maximum filling fraction  $1/4$ . Specifically, we employ our simulated annealing algorithm to obtain 10 configurations with  $N = 2400$  atoms at various filling fractions  $f = 0.245, 0.24, 0.23, 0.225, 0.22, 0.20$ , and  $0.16$ . As shown in Fig. S1, the structure factor for the dimers,  $S(k)$ , approaches a small value as  $k$  goes to zero, and the ensemble-averaged  $\sigma^2(R)/R^2$  decreases for large  $R$  at  $f$  close to  $1/4$ , which suggest possible effective hyperuniformity of these systems. To further quantify the degree of hyperuniformity at different  $f$ , we compute the ratio  $B/A$  described in the main text from the local number variance. As illustrated in Fig. S1(c), the ratio  $B/A$  increases for the monomer-dimer coverings as  $f$  approaches the maximum filling fraction  $1/4$ , indicating that the degree of hyperuniformity is increasing. Using a cutoff of  $B/A = 10$  for effective hyperuniformity, we deem dimer coverings to be effectively hyperuniform for filling fractions  $f \gtrsim 0.227$ .

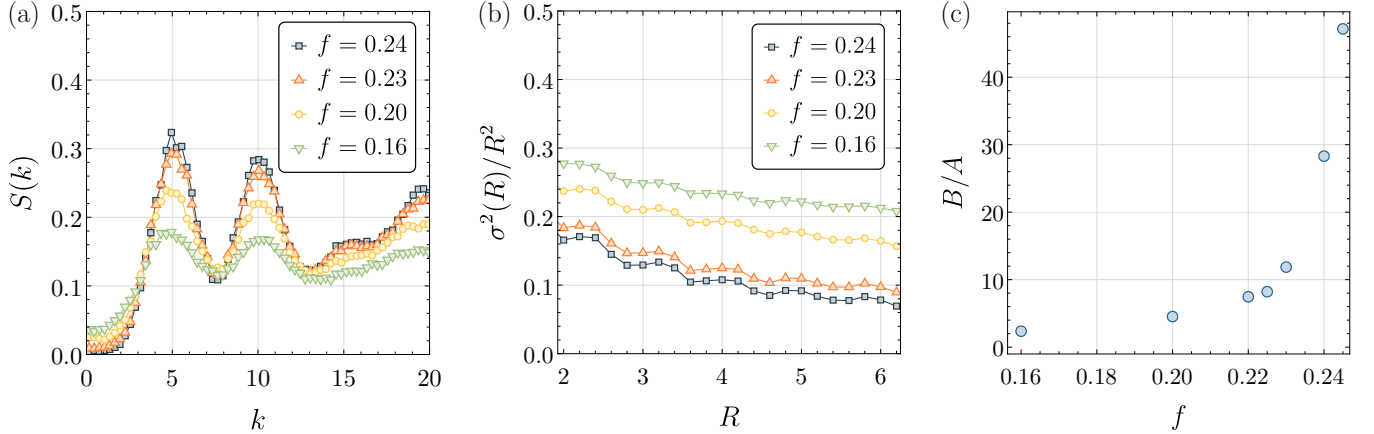

FIG. S1. (a) Structure factor  $S(k)$  and (b) local number variance  $\sigma^2(R)$  of the dimers (or equivalently, of Rydberg atoms in the excited state) with  $N = 2400$  total sites at different filling fractions  $f$ . The results are averaged over 10 configurations. (c) The ratio  $B/A$  of the parameters in the quadratic fitting  $f(R) = AR^2 + BR + C$  of the cumulative moving average  $\overline{\sigma^2(R)}$  of the number variance  $\sigma^2(R)$ , as a function of the filling fraction  $f$ .

\* These authors contributed equally to this work.

<sup>†</sup>Email: [torquato@electron.princeton.edu](mailto:torquato@electron.princeton.edu)

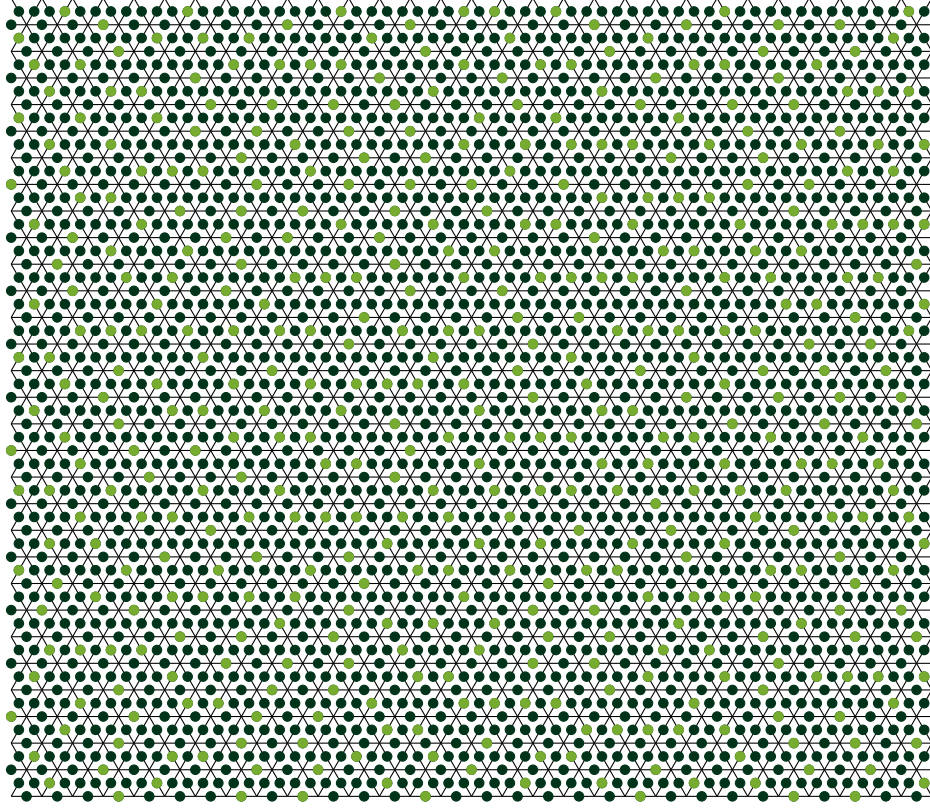

FIG. S2. A configuration of  $N = 2700$  atoms on the kagome lattice satisfying the dimer constraint, as generated by our simulated annealing algorithm. As before, light (dark) green circles represent an atom in the  $|r\rangle$  ( $|g\rangle$ ) state. Note that the configuration is apparently disordered and appears spatially uniform across length scales.

### PERFECT DIMER COVERINGS ON THE TRIANGULAR LATTICE

To determine the scaling exponent  $\alpha$  for perfect dimer liquids on the triangular lattice and their corresponding RK QSLs, we generate perfect dimer coverings at  $f = 1/6$  for various system sizes  $N = 1200, 1728, 2700, 3888$ , and  $4800$ . In Fig. S2, we show a representative example of a configuration of  $N = 2700$  atoms on the kagome lattice, which, once again, exhibits no apparent spatial symmetry-breaking order across length scales. We then compute the pair statistics of such perfect dimer coverings on the triangular lattice. In Fig. S3(a), we plot the ensemble-averaged structure factor  $S(k)$  of the dimer centers (for a few representative system sizes  $N = 1200, 2700, 4800$ ), which clearly approaches zero as  $k$  goes to zero, indicating perfect hyperuniformity of the perfect dimer coverings. Next, in Fig. S3(b), we present the corresponding ensemble-averaged local number variance  $\sigma^2(R)$ , which scales linearly as  $R$  increases and further demonstrates that perfect dimer coverings are class-I hyperuniform. We also determine the dimer-dimer pair correlation function  $C(r)$  for the system size  $N = 4800$ , and the result is shown in Fig. S3(c). Similarly to the case of perfect dimer coverings on the kagome lattice,  $C(r)$  decays to its long-range value of zero very rapidly as  $r$  increases, which is consistent with the theoretical expectation of exponential dimer correlations in the gapped  $\mathbb{Z}_2$  RVB liquid [1]. As before, this suggests that the structure factor  $S(k)$  is analytic at the origin, and consequently, the small- $k$  scaling exponent  $\alpha$  of  $S(k)$  should be a non-negative even integer. We compute  $\alpha$  at various system sizes  $N$  as shown in Fig. S3(d), which numerically extrapolates to approximately 4 in the infinite-system limit; since  $\alpha$  has to be a non-negative even integer, we can conclude that  $\alpha = 4$  exactly for the small- $k$  scaling of  $S(k)$  of the perfect dimer coverings on the triangular lattice.

### LOCAL NUMBER VARIANCE SCALING FOR PERFECT DIMER COVERINGS

Here, we present our theoretical analysis to demonstrate that the spatial distribution of dimers in the classical monomer-free dimer model (i.e., at the maximum filling fraction) on a lattice is perfectly hyperuniform, using the

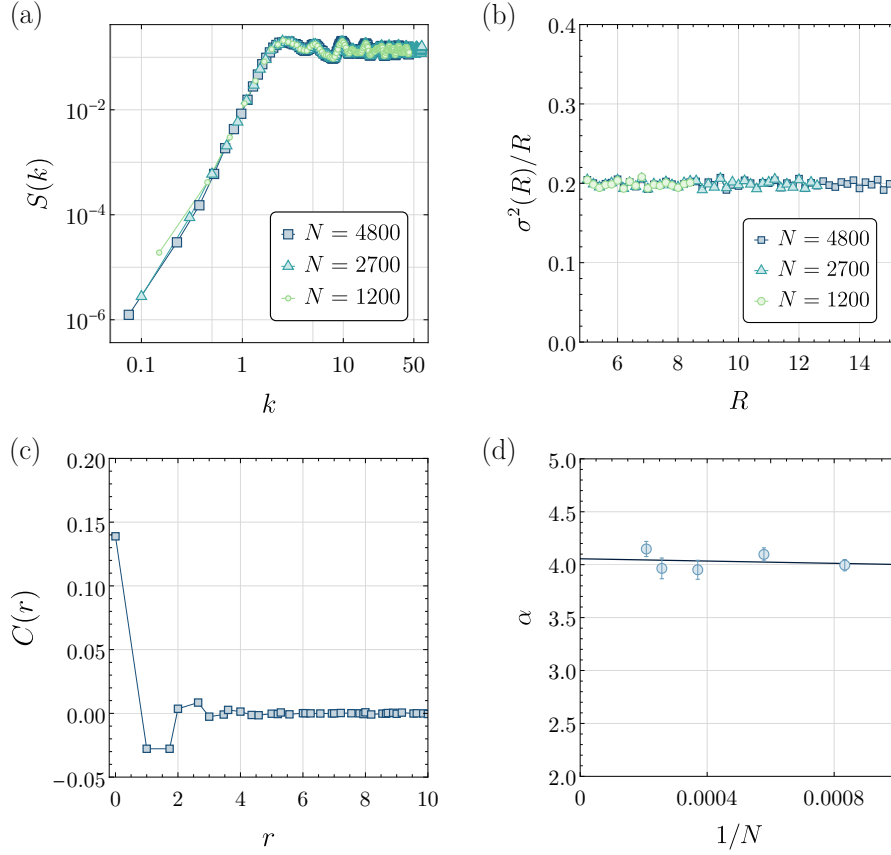

FIG. S3. (a) Ensemble-averaged structure factor  $S(k)$  and (b) local number variance  $\sigma^2(R)$  of perfect dimer coverings on the triangular lattice at different system sizes  $N$ . (c) Dimer-dimer pair correlation function  $C(r)$  of perfect dimer coverings on the triangular lattice at  $N = 4800$ . (d) Small- $k$  scaling exponent  $\alpha$  of  $S(k)$  as a function of inverse system size  $1/N$  for perfect dimer coverings on the triangular lattice. We work in units where the side length of a hexagon in the kagome lattice is set to be one.

dimer coverings on the kagome lattice at  $f = 1/4$  as an example. In particular, we link the density fluctuations of dimers to the density fluctuations of the kagome crystal through a “mass redistribution” process. Specifically, we divide the mass of each dimer in half, and transfer one half of the mass of this dimer to each of the two kagome vertices that it is touching, as depicted schematically in Fig. S4. Since each kagome vertex is touching exactly one dimer, and each dimer is touching exactly two kagome vertices, as a result of this mass redistribution, each kagome vertex has a particle with mass a half. To quantify the density fluctuation of the dimers, we randomly throw circular observation windows with radius  $R$  into the system, and count the number of dimers that fall within each observation window. For each observation window, before and after the mass redistribution, the number of dimers that fall within it only changes at the surface, i.e.,

$$\mathcal{N}_d(R) = \frac{1}{2}\mathcal{N}_k(R) + \varepsilon, \quad (\text{S1})$$

where  $\mathcal{N}_d(R)$  and  $\mathcal{N}_k(R)$  are the number of dimers and the number of kagome sites that fall within the window, respectively, and the change  $\varepsilon$  includes two *surface* contributions: i) a dimer is within the observation window, but at least one of its corresponding kagome sites is outside; ii) a dimer is outside the observation window, but at least one of its associated kagome vertices lies within. From classical results on the grand-canonical ensemble, the variance  $\sigma_\varepsilon^2(R)$  of  $\varepsilon$  should be proportional to the number of dimers  $\mathcal{N}_{d,s}$  in the vicinity of the window surface, i.e.,

$$\sigma_\varepsilon^2(R) \propto \mathcal{N}_{d,s} \propto R. \quad (\text{S2})$$

As a result, the local number variance  $\sigma_{\mathcal{N},d}^2(R)$  associated with  $\mathcal{N}_d(R)$  at large  $R$  is given by

$$\sigma_{\mathcal{N},d}^2(R) \approx \frac{1}{4}\sigma_{\mathcal{N},k}^2(R) + \sigma_\varepsilon^2(R) = \frac{1}{4}\sigma_{\mathcal{N},k}^2(R) + \mathcal{O}(R) \propto R, \quad (\text{S3})$$

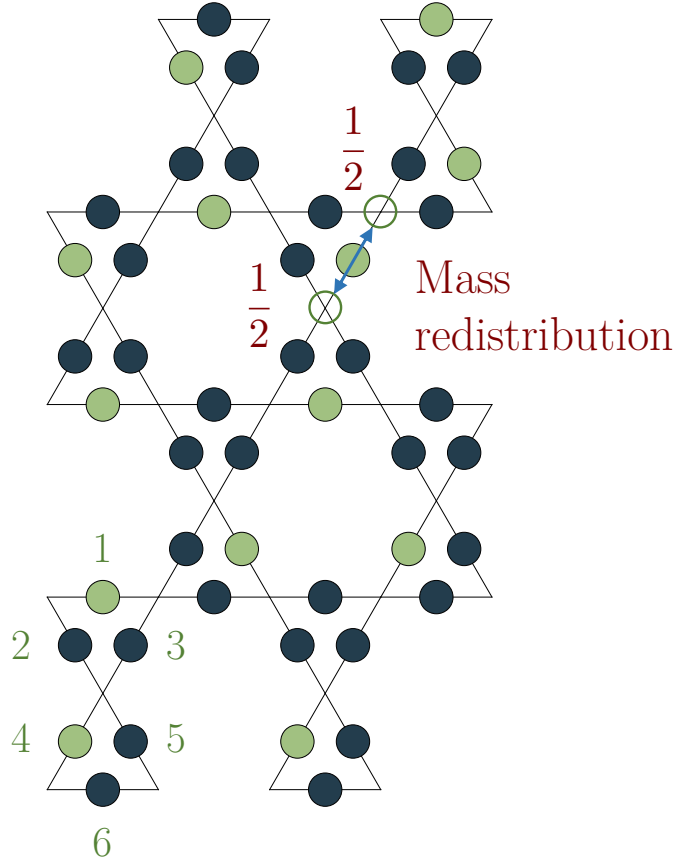

FIG. S4. Illustration of the “mass redistribution” idea, which is central to our theoretical analysis of the density fluctuations of perfect dimer coverings, illustrated here for the kagome-lattice dimer model. The numbering in the lower-left corner illustrates the local topology of two triangles that share a common vertex in the kagome lattice such that the dimer-dimer correlation function  $C(\mathbf{r})$  is nonzero.

where  $\sigma_{\mathcal{N},k}^2(R)$  is the local number variance of the kagome crystal, which is well known to scale linearly as  $R$  increases at large  $R$  [2, 3]. Hence, the distribution of the dimers is class-I hyperuniform. In Fig. S5 we visualize only the dimers (or atoms in the excited state) in a perfect dimer covering to highlight the disordered nature of the dimer distribution in a classical spin liquid phase.

#### CALCULATION OF STRUCTURE FACTOR AND LOCAL NUMBER VARIANCE

For particle configurations on lattice sites, which can be mapped to dimer coverings, the structure factor  $S(\mathbf{k})$  is given by

$$\begin{aligned}
 S(\mathbf{k}) &= \frac{1}{N} \sum_{i,j=1}^N (\langle n_i n_j \rangle - \langle n_i \rangle \langle n_j \rangle) \exp(-i\mathbf{k} \cdot \mathbf{r}_{ij}) \\
 &= \frac{1}{N} \sum_{i,j=1}^N \langle n_i n_j \rangle \exp(-i\mathbf{k} \cdot \mathbf{r}_{ij}) - \frac{1}{N} \sum_{i,j=1}^N \langle n_i \rangle \langle n_j \rangle \exp(-i\mathbf{k} \cdot \mathbf{r}_{ij})
 \end{aligned} \tag{S4}$$

where  $N$  is the number of lattice sites,  $n_i = 1$  indicates that lattice site  $i$  is occupied and  $n_i = 0$  otherwise, and  $\langle \dots \rangle$  denotes ensemble averaging. Here, we show that  $S(\mathbf{k})$  can be computed using the collective coordinate method.

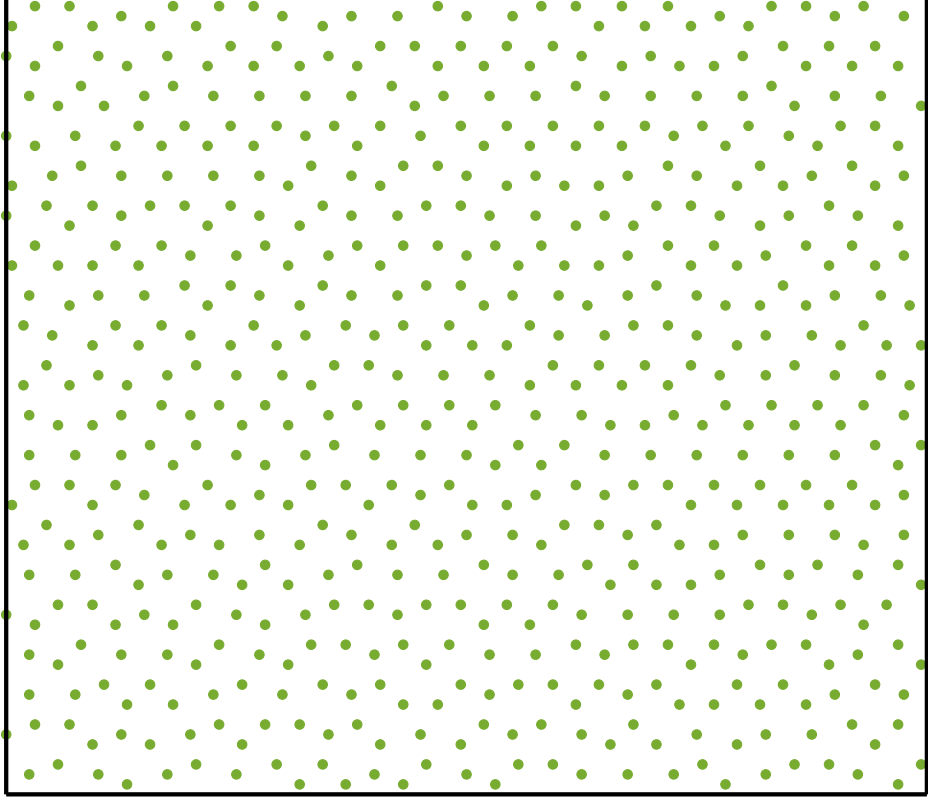

FIG. S5. A visualization showing only the dimers (or atoms in the excited state) in a perfect dimer covering on the kagome lattice. Note that the configuration is apparently disordered and appears spatially uniform across length scales.

Specifically, the first term in  $S(\mathbf{k})$  is given by

$$\begin{aligned}
 \frac{1}{N} \sum_{i,j=1}^N \langle n_i n_j \rangle \exp(-i\mathbf{k} \cdot \mathbf{r}_{ij}) &= \frac{1}{N} \sum_{i,j=1}^N \left( \frac{1}{\mathcal{D}} \sum_{\alpha=1}^{\mathcal{D}} n_{i,\alpha} n_{j,\alpha} \right) \exp(-i\mathbf{k} \cdot \mathbf{r}_{ij}) \\
 &= \frac{1}{\mathcal{D}} \sum_{\alpha=1}^{\mathcal{D}} \frac{1}{N} \left( \sum_{i,j=1}^N \exp(-i\mathbf{k} \cdot \mathbf{r}_{ij}) n_{i,\alpha} n_{j,\alpha} \right) \\
 &= \frac{1}{\mathcal{D}} \sum_{\alpha=1}^{\mathcal{D}} \frac{1}{N} \left( \sum_{i=1}^N \exp(i\mathbf{k} \cdot \mathbf{r}_i) n_{i,\alpha} \right) \left( \sum_{j=1}^N \exp(-i\mathbf{k} \cdot \mathbf{r}_j) n_{j,\alpha} \right) \\
 &= \frac{1}{\mathcal{D}} \sum_{\alpha=1}^{\mathcal{D}} \frac{1}{N} \left| \sum_{i=1}^N \exp(i\mathbf{k} \cdot \mathbf{r}_i) n_{i,\alpha} \right|^2 \\
 &= \frac{1}{\mathcal{D}} \sum_{\alpha=1}^{\mathcal{D}} \frac{1}{N} \left| \sum_{i=1}^{N_{e,\alpha}} \exp(i\mathbf{k} \cdot \mathbf{r}_{i,\alpha}) \right|^2,
 \end{aligned} \tag{S5}$$

where  $\mathcal{D}$  is the number of configurations in the ensemble (or states contributing to the quantum superposition),  $N_{e,\alpha} = N f_\alpha$  is the number of atoms in the excited state—or the number of dimers—in configuration  $\alpha$ ,  $f_\alpha$  is the filling fraction of configuration  $\alpha$ , and  $\mathbf{r}_{i,\alpha}$  denotes the coordinates of an occupied site  $i$  in configuration  $\alpha$ . Similarly,

the second term in  $S(\mathbf{k})$  is given by

$$\begin{aligned} \frac{1}{N} \sum_{i,j=1}^N \langle n_i \rangle \langle n_j \rangle \exp(-i\mathbf{k} \cdot \mathbf{r}_{ij}) &= \frac{1}{N} \left( \sum_{i=1}^N \exp(i\mathbf{k} \cdot \mathbf{r}_i) \langle n_i \rangle \right) \left( \sum_{j=1}^N \exp(-i\mathbf{k} \cdot \mathbf{r}_j) \langle n_j \rangle \right) \\ &= \frac{1}{N} \left| \sum_{i=1}^N \exp(i\mathbf{k} \cdot \mathbf{r}_i) \langle n_i \rangle \right|^2. \end{aligned} \quad (\text{S6})$$

Therefore,  $S(\mathbf{k})$  can be computed as

$$S(\mathbf{k}) = \frac{1}{\mathcal{D}} \sum_{\alpha=1}^{\mathcal{D}} \frac{1}{N} \left| \sum_{i=1}^{N_{e,\alpha}} \exp(i\mathbf{k} \cdot \mathbf{r}_{i,\alpha}) \right|^2 - \frac{1}{N} \left| \sum_{i=1}^N \exp(i\mathbf{k} \cdot \mathbf{r}_i) \langle n_i \rangle \right|^2. \quad (\text{S7})$$

For classical dimer coverings at a fixed filling fraction  $f$ , given the statistical homogeneity  $\langle n_i \rangle = f$ , the expression for  $S(\mathbf{k})$  can be further simplified as

$$S(\mathbf{k}) = \frac{1}{\mathcal{D}} \sum_{\alpha=1}^{\mathcal{D}} \frac{1}{N} \left| \sum_{i=1}^{N_{e,\alpha}} \exp(i\mathbf{k} \cdot \mathbf{r}_{i,\alpha}) \right|^2 - f^2 \frac{1}{N} \left| \sum_{i=1}^N \exp(i\mathbf{k} \cdot \mathbf{r}_i) \right|^2. \quad (\text{S8})$$

Subsequently,  $S(\mathbf{k})$  can be angular-averaged to obtain  $S(k)$ , where  $k = |\mathbf{k}|$ .

To compute the local number variance  $\sigma^2(R)$ , we randomly place circular observation windows with radius  $R$  at different locations in different configurations, and count the number of dimers (or atoms in the excited state)  $\mathcal{N}(R)$  that fall into the observation window, which is a random variable. The variance associated with  $\mathcal{N}(R)$  is denoted by  $\sigma^2(R) \equiv \langle \mathcal{N}(R)^2 \rangle - \langle \mathcal{N}(R) \rangle^2$ , which measures density fluctuations of particles within a window of radius  $R$ . Due to the quantum fluctuations, the total number of atoms in the excited state, i.e., the total number of dimers, differs across configurations, and we first average different locations to obtain a variance for each configuration and then average over different configurations when computing  $\sigma^2(R)$ . Specifically,  $\sigma^2(R)$  is given by

$$\sigma^2(R) = \frac{1}{\mathcal{D}} \sum_{i=1}^{\mathcal{D}} \left[ \frac{1}{w} \sum_{j=1}^w \mathcal{N}_{ij}^2(R) - \left( \frac{1}{w} \sum_{j=1}^w \mathcal{N}_{ij}(R) \right)^2 \right], \quad (\text{S9})$$

where  $w$  is the number of circular observation windows with radius  $R$  thrown into each of the snapshots ( $w \gg 1$ ), with the window locations the same for each configuration. Let  $\mathcal{N}_{i,j}(R)$  be the number of (excited) particles in configuration  $i$  that fall within the  $j$ -th window, which is one realization of the random number  $\mathcal{N}(R)$ . In addition, for quantum or classical systems with open boundary conditions in the horizontal direction and periodic boundary conditions in the vertical direction, when randomly placing observation windows into the systems, we restrict the windows to lie entirely within the range of  $[0.2L_x, 0.8L_x]$  in the horizontal direction (i.e., the interior of the simulation box) to avoid boundary artefacts, where  $L_x$  is the length of the simulation box in the horizontal direction.

## NUMERICAL CALCULATION OF $\alpha$

In this work, when computing the small- $k$  scaling exponent  $\alpha$  of  $S(k)$ , we first compute the excess spreadability  $\mathcal{S}(\infty) - \mathcal{S}(t)$  [4] at time  $t$  for point particles, which is linked to the spectral density  $\tilde{\chi}_V(\mathbf{k}) = \rho \tilde{m}^2(\mathbf{k}) S(k)$  via

$$\mathcal{S}(\infty) - \mathcal{S}(t) = \frac{1}{(2\pi)^d \phi_2} \int_{\mathbb{R}^d} \tilde{\chi}_V(\mathbf{k}) \exp[-k^2 D t] d\mathbf{k}, \quad (\text{S10})$$

where  $\rho$  is the particle number density of the system (which is a constant),  $d$  is the spatial dimension,  $D$  is the diffusion coefficient (which is set to unity),  $\phi_2$  is the volume fraction of the space unoccupied by the particles, and  $\tilde{m}(\mathbf{k})$  is the indicator function of a particle. When the particle size is negligibly small compared to the distance between neighboring particles, as in all cases considered in this work,  $\tilde{m}(\mathbf{k})$  is a constant, and we can replace  $\tilde{\chi}_V(\mathbf{k})$  with  $S(\mathbf{k})$ . For nonstealthy hyperuniform systems, a scaling of  $k^\alpha$  for  $S(k)$  at small  $k$  will translate into a scaling



$\mathcal{S}(\infty) - \mathcal{S}(t) \sim t^{-\varphi}$  at large  $t$  [4], where  $\varphi = (d + \alpha)/2$ . Subsequently, we extract the large- $t$  exponent  $\varphi$  of  $\mathcal{S}(\infty) - \mathcal{S}(t)$ , and the exponent  $\alpha$  is then computed as  $\alpha = 2\varphi - d$ . Since  $\mathcal{S}(\infty) - \mathcal{S}(t)$  can be essentially viewed as applying a Gaussian filter to  $S(k)$  to smooth the curve (i.e.,  $\mathcal{S}(\infty) - \mathcal{S}(t)$  at large  $t$  is smoother than  $S(k)$  at small  $k$ ), we find that the value of  $\alpha$  extracted this way is numerically more accurate than that obtained by directly fitting  $S(k)$  at small  $k$ .

## SCALING EXPONENT FOR PERFECT DIMER COVERINGS OF THE KAGOME LATTICE

In this section, we outline a theoretical proof that the small- $k$  scaling exponent  $\alpha$  in  $S(k) \sim k^\alpha$  is exactly 6 for perfect dimer coverings of the kagome lattice. We note that in computing  $S(k)$  numerically in the main text, we implicitly assume that we can perform an angular average of  $S(\mathbf{k})$  to obtain the radial function  $S(k)$ . In the following proof, it will become clear why this assumption is valid. As noted in the main text, since  $C(\mathbf{r})$  is short-ranged with compact support, it immediately follows that  $S(k)$  must be analytic at the origin, implying that the Taylor series of  $S(k)$  around  $k = 0$  can only involve even powers of  $k$ , i.e., the exponent  $\alpha$  should be a non-negative even integer.

Specifically, due to the constraint that each vertex in the kagome lattice is touched by exactly one dimer at the maximum filling fraction  $f = 1/4$ , and the fact that the dimer-dimer correlations are known to be exactly zero—in the infinite-system limit—for a pair of dimers when their corresponding triangles do not share a common vertex [5], the value of  $C(\mathbf{r})$  at each vector displacement  $\mathbf{r}$  is uniquely determined. We now explicitly show how we compute the two-point correlation function,  $C(\mathbf{r}) \equiv \langle n(\mathbf{x})n(\mathbf{x} + \mathbf{r}) \rangle - \langle n(\mathbf{x}) \rangle^2$ , where  $n(\mathbf{x})$  denotes the state of the occupation at position  $\mathbf{x}$ , which takes the value 1 if the site is occupied by a dimer and 0 otherwise, and  $\langle \dots \rangle$  denotes an ensemble and volume average over a single ensemble member. For vector displacements with magnitude  $r = 0$ ,  $C(\mathbf{r}) = f - f^2 = 3/16$  for  $f = 1/4$ . Next, when  $r = 1/2, \sqrt{3}/2$ , and 1,  $\langle n(\mathbf{x})n(\mathbf{x} + \mathbf{r}) \rangle = 0$  (as the direct result of the constraint that each kagome vertex is touched by at most one dimer), and for  $f = 1/4$ ,  $-\langle n(\mathbf{x}) \rangle^2 = -(1/4)^2 = -1/16$ ; thus  $C(\mathbf{r}) = -1/16$  for these displacements. For those vector displacements with  $r = \sqrt{7}/2$ , as illustrated by edges 1 and 4 (or 5) in a representative example shown in Fig. S4, when edge 1 is occupied, due to the dimer constraint, edges 2 and 3 cannot be occupied, and only one of edges 4 and 5 is occupied, leading to  $\langle n(\mathbf{x})n(\mathbf{x} + \mathbf{r}) \rangle = \frac{1}{4} \times \frac{1}{2} = \frac{1}{8}$  and  $C(\mathbf{r}) = \frac{1}{8} - \frac{1}{16} = \frac{1}{16}$ . Here, the factor  $\frac{1}{4}$  appears because, on average, every site has a probability of  $\frac{1}{4}$  to be occupied, and the factor  $\frac{1}{2}$  arises because only one of the two edges (4 and 5) that are  $r = \sqrt{7}/2$  away from an occupied site (edge 1) is occupied. Similarly, we can consider sites separated by a displacement of  $r = \sqrt{3}$ , which correspond to two edges in two triangles sharing a common vertex, e.g., edges 1 and 6 in Fig. S4: when edge 1 is occupied, edge 4 or 5 will be occupied, which prohibits the occupation of edge 6, leading to  $\langle n(\mathbf{x})n(\mathbf{x} + \mathbf{r}) \rangle = 0$  and  $C(\mathbf{r}) = 0 - \frac{1}{16} = -\frac{1}{16}$ . In Table I, we list all vector displacements where  $C(\mathbf{r})$  is not zero. Additionally,  $C(\mathbf{r})$  is zero for vector displacements with  $r = 3/2$  and  $r \geq \sqrt{13}/2$ , since these correspond to pairs of edges that do not belong to two triangles sharing a common vertex.

By grouping  $(i, j)$  pairs that correspond to the same  $\mathbf{r}$  in (S4), one can express  $S(\mathbf{k})$  as

$$S(\mathbf{k}) = \frac{1}{N} \sum_{\mathbf{r}} N_{\text{pair}}(\mathbf{r}) C(\mathbf{r}) \exp(-i\mathbf{k} \cdot \mathbf{r}). \quad (\text{S11})$$

We then insert all the listed nonzero values of  $C(\mathbf{r})$  in Table I, and obtain the analytical expression of  $S(\mathbf{k})$  as a finite sum. For  $\mathbf{k} = (k_x, k_y)$  with small  $k = |\mathbf{k}|$ , we can perform a Taylor expansion of  $S(\mathbf{k})$  in terms of  $k_x$  and  $k_y$ , and obtain the small- $k$  asymptotic formula:

$$S(\mathbf{k}) = \frac{3}{16384} k_x^6 + \frac{9}{32768} k_y^6 + \frac{45}{32768} k_x^4 k_y^2 + \mathcal{O}(k_x^2 k_y^6) + \mathcal{O}(k_x^4 k_y^4) + \mathcal{O}(k_x^6 k_y^2) + \mathcal{O}(k_x^8) + \mathcal{O}(k_y^8), \quad (\text{S12})$$

where  $\mathcal{O}(k_x^2 k_y^6)$ ,  $\mathcal{O}(k_x^4 k_y^4)$ ,  $\mathcal{O}(k_x^6 k_y^2)$ ,  $\mathcal{O}(k_x^8)$  and  $\mathcal{O}(k_y^8)$  represent all terms with order higher than or equal to  $k_x^2 k_y^6$ ,  $k_x^4 k_y^4$ ,  $k_x^6 k_y^2$ ,  $k_x^8$ , and  $k_y^8$ , respectively. Now, we switch to polar coordinates (i.e., substitute  $k_x$  and  $k_y$  with  $k \cos \theta$  and  $k \sin \theta$ , respectively, where  $k = |\mathbf{k}|$  is the wavenumber and  $\theta$  is the polar angle), and perform an angular average of  $S(\mathbf{k})$  to obtain  $S(k)$ :

$$\begin{aligned} S(k) &= \frac{1}{2\pi} \int_0^{2\pi} \left[ \frac{3}{16384} (k \cos \theta)^6 + \frac{9}{32768} (k \sin \theta)^6 + \frac{45}{32768} (k \cos \theta)^4 (k \sin \theta)^2 \right] d\theta + \mathcal{O}(k^8) \\ &= \frac{15}{65536} k^6 + \mathcal{O}(k^8) \end{aligned} \quad (\text{S13})$$

Our numerical results in the main text are consistent with the analytical expression in (S13), up to finite-size effects and the radial binning of  $k$  in the numerically calculated  $S(k)$ .

TABLE I. Values of the dimer-dimer correlation function  $C(\mathbf{r})$  and the corresponding number of edge pairs  $N_{\text{pair}}(\mathbf{r})$  (normalized by the number of lattice sites  $N$ ) at different vector displacements  $\mathbf{r}$  where  $C(\mathbf{r})$  is nonzero. Moreover,  $C(\mathbf{r})$  is zero for vector displacements with  $r = 3/2$  and  $r \geq \sqrt{13}/2$ . We additionally note that for rows marked with “\*”, we only count the pairs of edges at the corresponding vector displacements that belong to two triangles sharing a common vertex; there also exist edge pairs at the same vector displacements for which their associated triangles do not share a common vertex, and  $C(\mathbf{r}) = 0$  for these edge pairs.

| $\mathbf{r}$              | $r$          | $N_{\text{pair}}(\mathbf{r})/N$ | $C(\mathbf{r})$ |
|---------------------------|--------------|---------------------------------|-----------------|
| (0,0)                     | 0            | 1                               | 3/16            |
| $\pm(1/2, 0)$             | 1/2          | 1/3                             | -1/16           |
| $\pm(1/4, \sqrt{3}/4)$    | 1/2          | 1/3                             | -1/16           |
| $\pm(-1/4, \sqrt{3}/4)$   | 1/2          | 1/3                             | -1/16           |
| $\pm(0, \sqrt{3}/2)$      | $\sqrt{3}/2$ | 1/3                             | -1/16           |
| $\pm(3/4, \sqrt{3}/4)$    | $\sqrt{3}/2$ | 1/3                             | -1/16           |
| $\pm(-3/4, \sqrt{3}/4)$   | $\sqrt{3}/2$ | 1/3                             | -1/16           |
| $\pm(1, 0)$               | 1            | 1/3                             | -1/16           |
| $\pm(1/2, \sqrt{3}/2)$    | 1            | 1/3                             | -1/16           |
| $\pm(-1/2, \sqrt{3}/2)$   | 1            | 1/3                             | -1/16           |
| $\pm(-1/4, 3\sqrt{3}/4)$  | $\sqrt{7}/2$ | 1/3                             | 1/16            |
| $\pm(1/4, 3\sqrt{3}/4)$   | $\sqrt{7}/2$ | 1/3                             | 1/16            |
| $\pm(5/4, -\sqrt{3}/4)$   | $\sqrt{7}/2$ | 1/3                             | 1/16            |
| $\pm(-5/4, -\sqrt{3}/4)$  | $\sqrt{7}/2$ | 1/3                             | 1/16            |
| $\pm(1, \sqrt{3}/2)$      | $\sqrt{7}/2$ | 1/3                             | 1/16            |
| $\pm(-1, \sqrt{3}/2)$     | $\sqrt{7}/2$ | 1/3                             | 1/16            |
| $\pm(0, \sqrt{3})^*$      | $\sqrt{3}$   | 1/6                             | -1/16           |
| $\pm(3/2, \sqrt{3}/2)^*$  | $\sqrt{3}$   | 1/6                             | -1/16           |
| $\pm(3/2, -\sqrt{3}/2)^*$ | $\sqrt{3}$   | 1/6                             | -1/16           |

- 
- [1] R. Moessner and K. S. Raman, in *Introduction to Frustrated Magnetism* (Springer, 2011) pp. 437–479.
  - [2] S. Torquato and F. H. Stillinger, *Phys. Rev. E* **68**, 041113 (2003).
  - [3] S. Torquato, *Phys. Rep.* **745**, 1 (2018).
  - [4] H. Wang and S. Torquato, *Phys. Rev. Appl.* **17**, 034022 (2022).
  - [5] G. Misguich, D. Serban, and V. Pasquier, *Phys. Rev. Lett.* **89**, 137202 (2002).
